# Supplementary material for: Atomic nonaffinity as a predictor of plasticity in amorphous solids
Source: arXiv:1905.12035 source file (2021-02-04)
Supplement: Supplementary file 1 [file supplementary_materials.pdf]

# Supplementary Materials for "Atomic nonaffinity as a predictor of plasticity in amorphous solids"

Bin Xu, Michael L. Falk, Sylvain Patinet, and Pengfei Guan

## I. CLOSE TO INSTABILITY OF ONE PLASTIC EVENT

The two-dimensional system mentioned in the main text was sheared to be very close to the triggering strain of a plastic event via a protocol of athermal quasistatic shear. A plastic event will be triggered in the region (Fig. S1(a)) where the mode with lowest eigenvalue is localized, if the system were to be further sheared in the pre-sheared direction (the reference direction $\theta_{\mathrm{L}} = 0$). However, if the system were to be further sheared in other directions, such as $\theta_{\mathrm{L}} = \frac{\pi}{4}$, no plastic event would be observed in the region, as shown in Fig. S1(b), even when subjected to a large magnitude of strain.

## II. TRIGGERING STRAIN OF THE SOFTEST MODE

In athermal quasistatic shear (AQS), the system is always mechanically stable and must reside at a minimum on the energy landscape. The energy of system $U$ can be expanded with a third-order Taylor approximation based on the vibrational coordinate $q^*$ of the softest mode and shear strain as

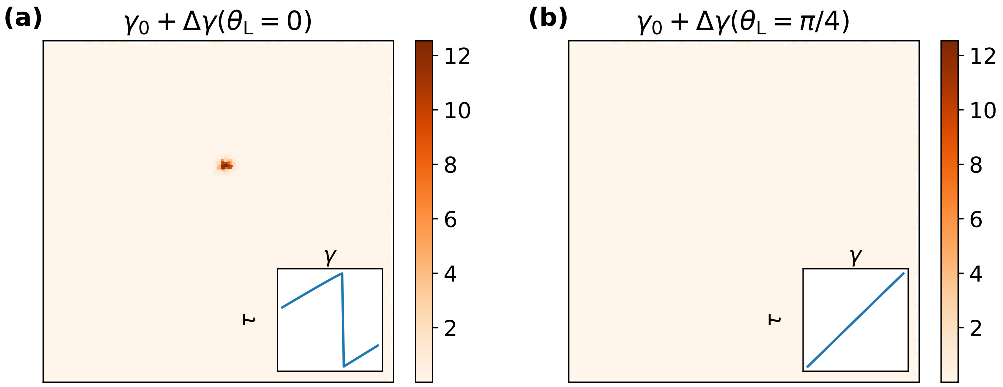


FIG. S1. The $D^2_{\mathrm{min}}$ field after simple shear with $\theta_{\mathrm{L}} = 0$ (a) and $\theta_{\mathrm{L}} = \pi/4$ (b). The loading shear strain was $6 \times 10^{-5}$. A plastic event was triggered when $\theta_{\mathrm{L}} = 0$.

$$U \approx U_0 + \frac{\partial U}{\partial \gamma}\Delta\gamma + \frac{1}{2}\frac{\partial^2 U}{\partial \gamma^2}\Delta\gamma^2 + \frac{\lambda^*}{2}\Delta q^{*2} + V\Delta\gamma\Delta q^*\frac{\partial \tau(\theta_\mathrm{L})}{\partial q^*} + \frac{\eta^*}{6}\Delta q^{*3}$$
$$+ \frac{1}{2}\frac{\partial^3 U}{\partial q^{*2}\partial\gamma}\Delta q^{*2}\Delta\gamma + \frac{1}{2}\frac{\partial^3 U}{\partial q^{*}\partial\gamma^2}\Delta q^{*}\Delta\gamma^2 + \frac{1}{6}\frac{\partial^3 U}{\partial\gamma^3}\Delta\gamma^3 \quad (1)$$

where $\lambda^*$ is the eigenvalue, $\eta^*$ is the third derivative of energy with respect to coordinate $q^*$, $V$ is the volume of the system, $\tau(\theta_\mathrm{L})$ is the shear stress in the shear orientation $\theta_\mathrm{L}$, and $\Delta\gamma = \gamma - \gamma_0$ is the shear strain. We can further formulate the following assumptions:

- Stress variation along vibrational coordinate $q^*$ is linear. Then, $\frac{\partial^3 U}{\partial q^{*2}\partial\gamma} = 0$.
- Affine shear modulus of system remains the same for different vibrational coordinate $q^*$. Then, $\frac{\partial^3 U}{\partial q^{*}\partial\gamma^2} = 0$.

The above assumptions are reasonable as observed in Ref. [1]. At $\gamma_0$, the initial minimum coordinate is $q_0^*$, and we set $q_0^* = 0$ to simplify the notation. Then, $\Delta q^* = q^* - q_0^* = q^*$. Two stationary points, the initial minimum and saddle point at strain $\Delta\gamma$, can be obtained by solving the following equation

$$\frac{\partial U}{\partial q^*} = \frac{\eta^*}{2}q^{*2} + \lambda^* q^* + V\Delta\gamma\frac{\partial \tau(\theta_\mathrm{L})}{\partial q^*} = 0. \quad (2)$$

At triggering strain $\Delta\gamma_c$, the two roots of Eq. (2) are equal, and

$$\Delta\gamma_c(\theta_\mathrm{L}) = \frac{\lambda^{*2}}{2\eta^* V\frac{\partial \tau(\theta_\mathrm{L})}{\partial q^*}}. \quad (3)$$

$\Delta\gamma_c(\theta_\mathrm{L})$ reaches minimum when $\frac{\partial \tau(\theta_\mathrm{L})}{\partial q^*}$ reaches maximum. This occurs when the corresponding orientation $\theta_\mathrm{L}$ equals to $\theta_s$, which is the softest shear orientation defined in the main text. From stress transformation rules, we can get

$$\frac{\partial \tau}{\partial q^*}(\theta_\mathrm{L}) = \frac{\partial \tau(\theta_s)}{\partial q^*}\cdot\cos[2(\theta_\mathrm{L} - \theta_s)]. \quad (4)$$

Finally, the relation between $\Delta\gamma_c$ and the angle can be written as

$$\Delta\gamma_c = \Delta\gamma_{c,\mathrm{min}}\cdot\cos[2(\theta_\mathrm{L} - \theta_s)]. \quad (5)$$

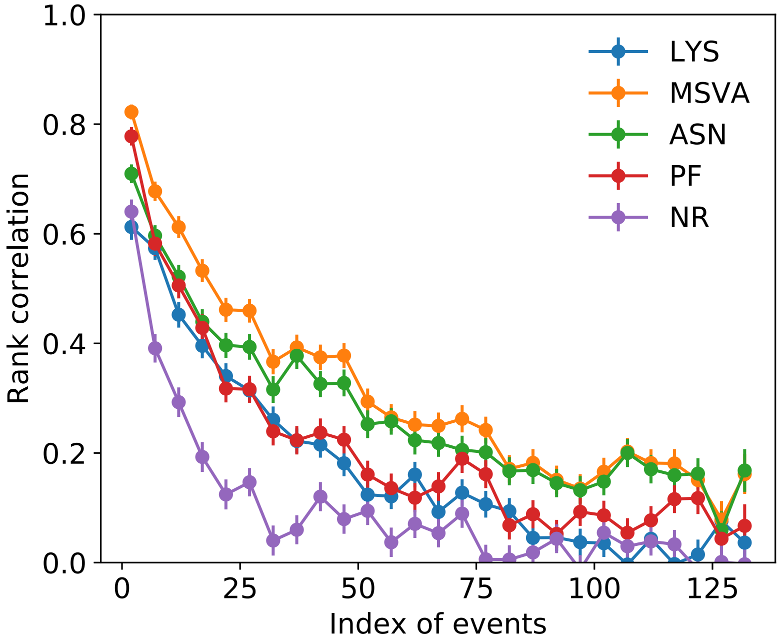


FIG. S2. Correlation between different indicators and the locations of plastic events as a function of index of events.

## III. PREDICTIVE POWER OF INDICATORS FOR CONFIGURATIONS INSTANTLY QUENCHED FROM HIGH TEMPERATURE LIQUIDS

In the main text, we show the predictive power of indicators for configurations prepared via a slow cooling rate from high temperature liquid. Here, we show the results for configurations prepared via instantly quenching from high temperature liquids (HTL) in Fig. S2. Different from the those slowly quenched configurations, MSVA and ASN have a better predictive power than the LYS. One possible reason for the big drop of predictive power of LYS is that the LYS is purely a local method. Its statistics is narrower for HTL and has the same order as the mechanical noise [2].

## IV. LOCATIONS OF PLASTIC EVENTS WITH DIFFERENT SHEAR PROTOCOLS

In the Fig. 2 of the main text, we show the correlation between $\theta_s$ calculated from the undeformed configuration and the locations of plastic events in shear protocols with $\theta_{\mathrm{L}} = 0$

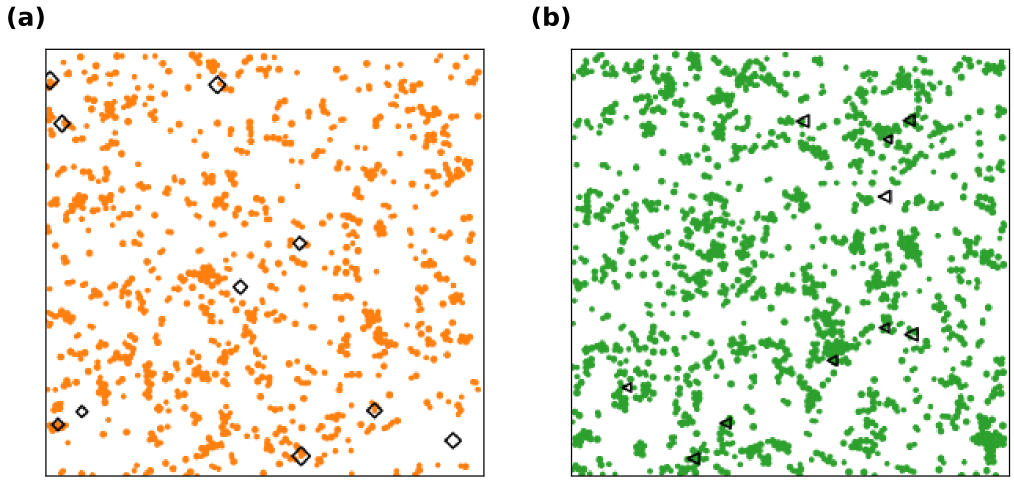


FIG. S3. (a) Orange circles represents the atom with $\mathrm{RC}_{\hat{G}} > 0$ and $\theta_s > 0$. Diamond mark the locations of the first ten plastic events with $\theta_\mathrm{L} = \frac{\pi}{4}$. (b) Green circles represents the atom with $\mathrm{RC}_{\hat{G}} > 0$ and $\theta_s < 0$. Triangles mark the locations of the first ten plastic with $\theta_\mathrm{L} = -\frac{\pi}{4}$.

and $\frac{\pi}{2}$. Here in Fig. S3, we show the results of the same configuration for two other shear protocols with $\theta_\mathrm{L} = \frac{\pi}{4}$ and $-\frac{\pi}{4}$. It was observed that core atoms of most events satisfied the condition $|\theta_s - \theta_\mathrm{L}| < \frac{\pi}{4}$ mentioned in the main text.

## V. STATISTICS FOR THE ROTATION OF THE SOFTEST SHEAR ORIENTATION

In the main text, we show that the distribution of the softest orientations is broadened when measured from the configuration associated with the previous event. Here, we show that the broadening effect is correlated with incremental triggering strain required to induce each event. As shown in Fig. S4(a), the fraction of the plastic events with orientations within the range $\theta_s(\mathrm{ID}_N, \gamma_{c,N-1,A}) - \theta_\mathrm{L} < \frac{\pi}{4}$ decreases from one to around 0.75. We also measure the distribution of the change of orientation for the core atoms for each plastic event since the triggering of the previous event, as shown in Fig. S4(b). The change of orientation for most events are small, but a few events do undergo large change of orientation.

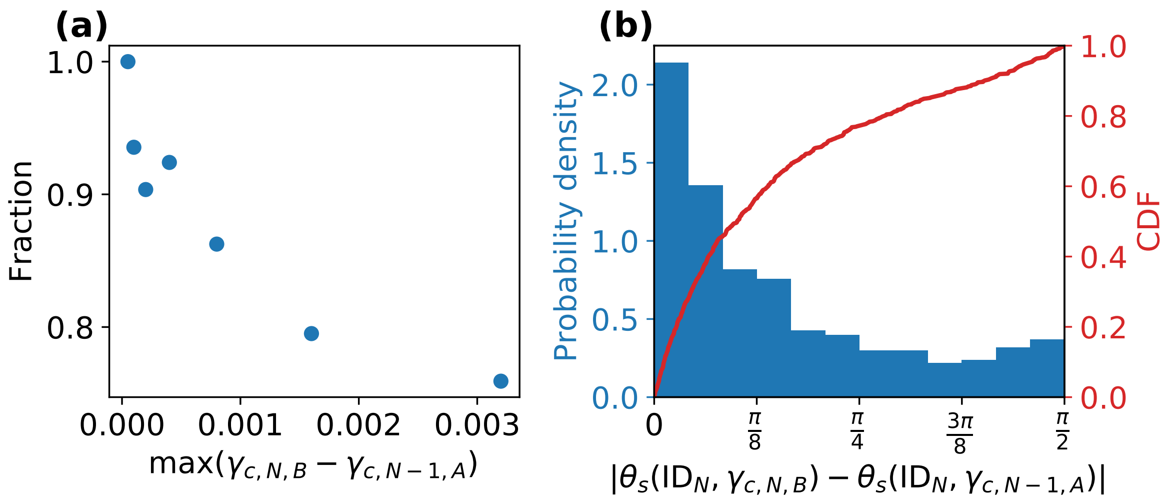


FIG. S4. (a) Measuring the broadening effect of distribution of orientation of plastic events at different strains intervals before triggering point. The fraction is the number fraction of events that satisfy $|\theta_s(\mathrm{ID}_N, \gamma_{c,N-1,A}) - \theta_\mathrm{L}| < \frac{\pi}{4}$. If one measure the orientations of the plastic events at a larger strain before the triggering point, the distribution of orientations will be more broaden. (b) The change of orientations if one measure the orientation of plastic events from the configurations after the triggering of previous event of each event and from the configuration just before the triggering of each event. Red line represents the commutative distribution function of the distribution.

## VI. IMPROVING THE PRECISION OF PREDICTION VIA CHARACTERIZING THE SOFTEST SHEAR ORIENTATION

As the plastic events tend to happen in STZs with the softest shear orientations close the orientation of shear protocols, one can expect that characterizing the softest shear orientations will help improve the predictive power of those indicators that do not contain orientational information. In Fig. S5, we show that the precision of predicting the location of core atoms for first events of 100 samples is improved by a factor close to 2 by filtering out those regions that do not have a good alignment with the orientations with the shear protocols. In the graph, the rank threshold means that the threshold to label the "softest" atoms characterized by different indicators as the potential locations of first plastic event of each sample. E.g. if rank threshold equals 10 for atomic shear shear nonaffinity, we label the atoms with the 10 lowest atomic shear nonaffinity as the potential locations of the first

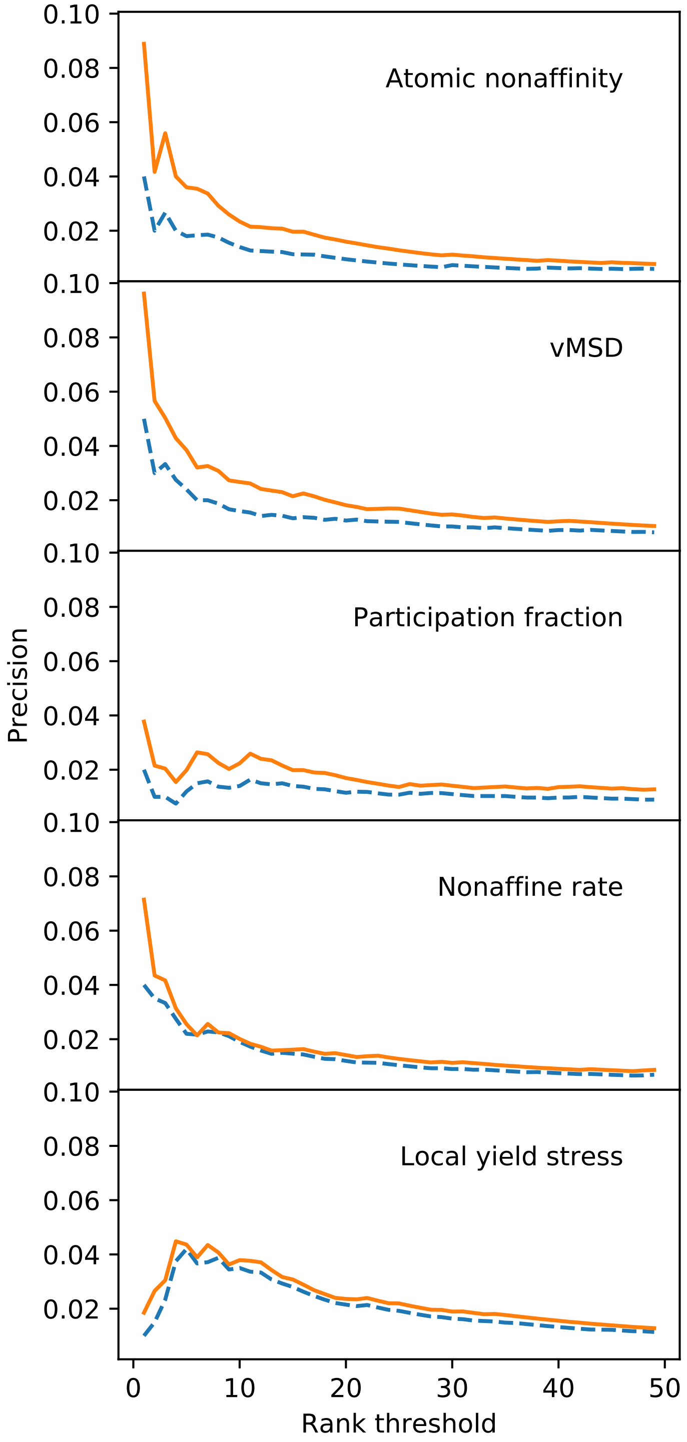


FIG. S5. Predictive precision of different indicators at different rank threshold. Dash blue lines represent results for single indicators. Solid orange lines represent results for each indicators after filtering the atoms with $|\theta_S - \theta_{\mathrm{L}}| < \pi/4$.

plastic events. For 100 samples we used here, we will totally label 1000 atoms. If in all labeled atoms, there are 30 atoms that are just the core atoms of the 100 first plastic event of 100 samples, the precision will be 30/1000 = 0.03, which is True Positive/ Total postive. After obtaining the softest shear orientational of each atom, for those 1000 labeled atoms, we filter those atoms with $|\theta_S - \theta_\mathrm{L}| < \pi/4$, since we estimate that only the plastic events will in most cases happen in those regions that have a good alignment with shear protocols. On average, 500 atoms will left after filtering, since the amorphous materials are statistically isotropic in the quench state. If all the true positive atoms are in the atoms left after filtering, the precision will be 30/500 = 0.06, where the precision will be improved by a factor of 2. In Fig. S5, the improving factor is close to 2 for small rank threshold but decay to smaller values as rank threshold increases.

## VII. A SIMPLE MODEL OF INDEPENDENT PLASTIC EVENTS WITH INTRINSIC ORIENTATIONS

In this section, we present a simple mean-field model of independent plastic events with intrinsic orientations to understand the distribution of orientations for triggered plastic events after shear deformation.

### A. Assumptions

- Each shear transformation zone (STZ) in an amorphous solid has two important and independent properties, i.e. the softest shear orientation (denoted as $\theta_{s,i}$) and the minimum triggering strain (denoted as $\gamma_{c,s,i}$). $\theta_{s,i}$ is confined in the range $[-\frac{\pi}{2}, \frac{\pi}{2})$ considering the symmetry of shear.

- The triggering strain for one STZ at a given imposed shear orientation (denoted as $\theta_\mathrm{L}$) may be expressed as

$$\gamma_{c,i}(\theta_\mathrm{L}) = \frac{\gamma_{c,s,i}}{\cos[2(\theta_{s,i} - \theta_\mathrm{L})]}. \quad (6)$$

- The initial microstructure of the amorphous solid is isotropic. Then, the number density of STZs with specified properties $\theta_s$ and $\gamma_{c,s}$ does not rely on the $\theta_s$, i.e.

$$\rho(\theta_s, \gamma_{c,s}) = \rho(\gamma_{c,s}), \quad (7)$$

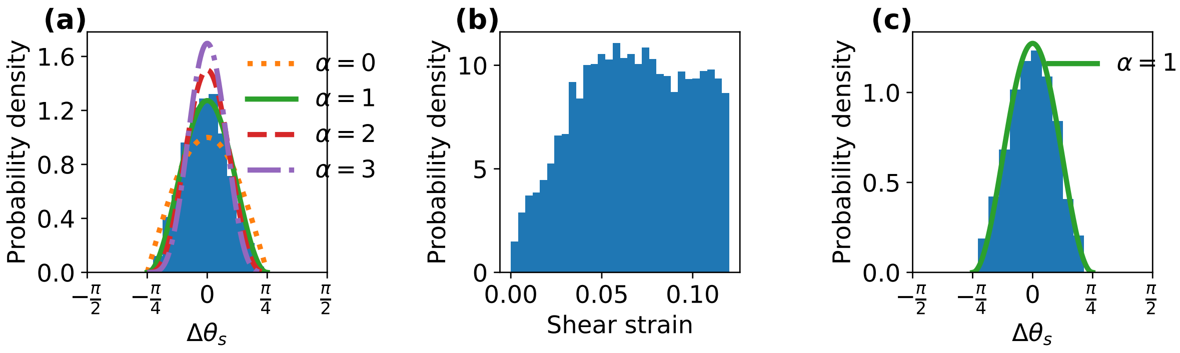


FIG. S6. (a) The distribution of the softest shear orientations for all the plastic events that are triggered before shear strain 0.12 in 10 samples. The softest shear orientations are measured based on the configuration just before the triggering of each event. Each line represents the predictions from Eqs. (11) and (12). (b) The probability density for the triggering strains for all the plastic events in AQS for 100 samples. (c) The distribution of the softest shear orientations for the first five events that are triggered in AQS for 100 samples. The softest shear orientations are measured based on the configuration just before the triggering of each event.

where $\rho$ is the number density.

- We further assume that $\rho(\gamma_{c,s})$ follows a power law, i.e. $\rho(\gamma_{c,s}) = A\gamma_{c,s}^{\alpha}$.

Noting that here we neglects that fact that when one STZ is activated upon deformation it may get a new orientation and new minimum triggering strain. This is reasonable when new triggering strain is large and plastic events are sparse, which is close to the situation of that the configurations are prepared with slow cooling rate and observing strain range is before yielding.

### B. Derivation of correlation between number density function and distribution of orientations of triggered events in one shear orientation

We set the orientation of shear protocol as the referential orientation with value of $\theta_{\mathrm{L}} = 0$, set the loading shear strain as $\gamma_{\mathrm{L}}$ and denote the total number of the plastic events with

$\gamma_{c,s} \le \gamma_{\mathrm{L}}$ as $N(\gamma_{\mathrm{L}})$. Then, we obtain

$$N(\gamma_{\mathrm{L}}) = \int_{\frac{\pi}{2}}^{-\frac{\pi}{2}} \int_{0}^{\gamma_{\mathrm{L}}} \rho(\gamma_{c,s})\, d\gamma_{c,s}\, d\theta_s = \pi \int_{0}^{\gamma_{\mathrm{L}}} \rho(\gamma_{c,s})\, d\gamma_{c,s} = \frac{A\pi}{\alpha+1}\gamma_{\mathrm{L}}^{\alpha+1}. \tag{8}$$

Then,

$$A = \frac{(\alpha+1)N(\gamma_{\mathrm{L}})}{\pi\gamma_{\mathrm{L}}^{\alpha+1}}. \tag{9}$$

For events with $|\theta_s| \le \frac{\pi}{4}$, only those events with condition that $\gamma_{c,s} \le \gamma_{\mathrm{L}} \cos 2\theta_s$ will triggered. Then, the number density ($\tilde{\rho}$) of events that are triggered with property $\theta_s$ is

$$\tilde{\rho}(\theta_s) = \int_{0}^{\gamma_{\mathrm{L}}\cos 2\theta_s} \rho(\gamma_{c,s})\, d\gamma_{c,s} = \frac{A}{\alpha+1}\gamma_{\mathrm{L}}^{\alpha+1}\cos^{\alpha+1} 2\theta_s = \frac{N(\gamma_{\mathrm{L}})}{\pi}\cos^{\alpha+1} 2\theta_s. \tag{10}$$

Events with $|\theta_s| > \frac{\pi}{4}$ will not be triggered in this protocol. Thus, the probability density ($\hat{\rho}(\theta_s)$) of events that are triggered should have the form

$$\hat{\rho}(\theta_s) = k\cos^{\alpha+1} 2\theta_s, \tag{11}$$

where $k$ is the normalizing factor that ensures that the total probability equals one. The peak probability corresponds to events that have the same orientation as the shear protocol i.e. $\theta_s = 0$, and $\hat{\rho}_{\max} = \hat{\rho}(\theta_s = 0) = k$. For different power-law factors, we infer the value of $k$ to be

$$\begin{aligned} \alpha &= 0,\ k = 1, \\ \alpha &= 1,\ k = \frac{4}{\pi} \approx 1.27, \\ \alpha &= 2,\ k = \frac{3}{2}, \\ \alpha &= 3,\ k = \frac{16}{3\pi} \approx 1.70. \end{aligned} \tag{12}$$

In the systems that we investigated in the main text, we found that $\hat{\rho}(\theta_s)$ corresponds closely to what would be expected from $\alpha = 1$, as shown in Fig. S6(a). When $\alpha = 1$, one can also derive that the probability density of triggering strains for the plastic events in AQS should be a linear function of shear strain; this was further verified in simulations as shown in Fig. S6(b). The function is close to linear relation before yielding, but a plateau arises after yielding. To confirm the linear regime we further checked the distribution of the softest orientations for the first five plastic in 100 samples. The distribution was also found to be

close to distribution of $\alpha = 1$, as shown in Fig. S6(c).

[1] B. Xu, M. Falk, J. Li, and L. Kong, Phyiscal Review B **95**, 144201 (2017).

[2] A. Barbot, M. Lerbinger, A. Hernandez-Garcia, R. García-García, M. L. Falk, D. Vandembroucq, and S. Patinet, Physical Review E **97**, 033001 (2018), arXiv:1802.05796.
